# Supplementary material for: CAT: Causal Audio Transformer for Audio Classification
Source: arXiv:2303.07626 source file (2023-03-14)
Supplement: Supplementary file 1 [file 6_appendix.tex]

\section{Appendix}
% \footnotesize
\label{app}
We derive the Equation~\ref{eq:final} as follows: the intervention distribution under a functional intervention $P(Y|do(f(X)=z))$ following \cite{puli2020causal} can be approximated as:
\begin{equation}
    \vspace{-2mm}
    \label{eq:intv}
    \footnotesize
    \int P(Y|do(X))P(X|C, f(X)=z)p(C)dXdC
\end{equation}
where $C$ is the unobserved confounder. 
The lower bound takes the form of the difference between two interventional probability $P(Y=y | do(X),C)$ and $P(Y=y | do(Z=z))$. Then we have:
\begin{equation}
\footnotesize
    \label{eq:first}
    P(Y=y | do(X)) = P(Y|X)
\end{equation}
\vspace{-5mm}
\begin{equation}
    \label{eq:second}
    \footnotesize
    P(Y=y | do(Z=z)) = \int P(X|C, f(X)=z) p(C)d(C)
\vspace{-1mm}
\end{equation}

Combining Equation~\ref{eq:first}, \ref{eq:second} and \ref{eq:intv}, we have
\begin{align*}
    \footnotesize
        &P(Y=y | do(Z=z)) \\
        &= \int P(Y|X) \cdot (\int P(X|C, f(X)=z) p(C)d(C)) dX \\
        &= \int P(Y|X) P(X|f(X)=z) dX
\end{align*}

Consequently, 
\begin{align*}
\footnotesize
    &P(Y=y | do(Z=z)) - P(Y=y | do(Z \neq z)) \\
    &= \int P(Y|X) [P(X|f(X)=z) - P(X|f(X)\neq z)] dX
\end{align*}
